# Supplementary material for: Can Machines Philosophize?
Source: arXiv:2507.00675 source file (2025-10-03)
Supplement: Supplementary file 1 [file supplementary.pdf]

# SUPPLEMENTARY INFORMATION

## Can Machines Philosophize?

### Simulating Humans' Views with AI Personas

Michele Pizzochero

*Department of Physics, University of Bath, Bath BA2 7AY, United Kingdom*

*School of Engineering and Applied Sciences, Harvard University, Cambridge, MA 02138, United States*

Giorgia Dellaferrera

*McKinsey & Company, London WC1A 1PB, United Kingdom*

#### List of Supplementary Tables

|          |                                 |    |
|----------|---------------------------------|----|
| <b>1</b> | Supplementary Table 1 . . . . . | 2  |
| <b>2</b> | Supplementary Table 2 . . . . . | 15 |

#### List of Supplementary Figures

|           |                                   |    |
|-----------|-----------------------------------|----|
| <b>1</b>  | Supplementary Figure 1 . . . . .  | 3  |
| <b>2</b>  | Supplementary Figure 2 . . . . .  | 4  |
| <b>3</b>  | Supplementary Figure 3 . . . . .  | 5  |
| <b>4</b>  | Supplementary Figure 4 . . . . .  | 6  |
| <b>5</b>  | Supplementary Figure 5 . . . . .  | 7  |
| <b>6</b>  | Supplementary Figure 6 . . . . .  | 8  |
| <b>7</b>  | Supplementary Figure 7 . . . . .  | 9  |
| <b>8</b>  | Supplementary Figure 8 . . . . .  | 10 |
| <b>9</b>  | Supplementary Figure 9 . . . . .  | 11 |
| <b>10</b> | Supplementary Figure 10 . . . . . | 12 |
| <b>11</b> | Supplementary Figure 11 . . . . . | 13 |
| <b>12</b> | Supplementary Figure 12 . . . . . | 14 |

|                | AGREEMENT SCORE, $\bar{s}$ (%) |                   |                   |                   |
|----------------|--------------------------------|-------------------|-------------------|-------------------|
|                | PHYSICISTS                     |                   | PHILOSOPHERS      |                   |
| STATEMENT, $S$ | Human                          | Machine           | Human             | Machine           |
| 1              | 65.00 $\pm$ 29.10              | 57.47 $\pm$ 23.39 | 59.07 $\pm$ 27.72 | 58.92 $\pm$ 26.88 |
| 2              | 79.42 $\pm$ 21.42              | 71.21 $\pm$ 15.75 | 68.22 $\pm$ 24.88 | 61.63 $\pm$ 20.53 |
| 3              | 39.43 $\pm$ 32.64              | 43.52 $\pm$ 12.63 | 43.48 $\pm$ 30.64 | 38.95 $\pm$ 14.74 |
| 4              | 80.40 $\pm$ 23.26              | 71.54 $\pm$ 9.81  | 72.25 $\pm$ 26.76 | 63.08 $\pm$ 14.15 |
| 5              | 29.59 $\pm$ 28.88              | 36.96 $\pm$ 11.10 | 32.76 $\pm$ 28.49 | 35.57 $\pm$ 12.76 |
| 6              | 71.75 $\pm$ 26.66              | 61.35 $\pm$ 10.72 | 68.52 $\pm$ 25.47 | 54.83 $\pm$ 12.40 |
| 7              | 46.44 $\pm$ 30.69              | 50.47 $\pm$ 10.02 | 40.99 $\pm$ 31.64 | 49.00 $\pm$ 11.61 |
| 8              | 74.00 $\pm$ 24.83              | 71.70 $\pm$ 8.88  | 68.67 $\pm$ 26.14 | 64.72 $\pm$ 16.11 |
| 9              | 46.09 $\pm$ 32.18              | 44.98 $\pm$ 14.04 | 42.14 $\pm$ 31.67 | 38.85 $\pm$ 17.09 |
| 10             | 49.95 $\pm$ 30.49              | 53.47 $\pm$ 14.32 | 53.35 $\pm$ 30.08 | 47.60 $\pm$ 17.13 |
| 11             | 76.94 $\pm$ 23.50              | 62.43 $\pm$ 11.84 | 62.98 $\pm$ 28.37 | 56.53 $\pm$ 13.98 |
| 12             | 51.48 $\pm$ 30.16              | 57.99 $\pm$ 13.43 | 61.96 $\pm$ 25.83 | 56.47 $\pm$ 14.20 |
| 13             | 85.39 $\pm$ 21.35              | 85.09 $\pm$ 8.31  | 80.82 $\pm$ 22.11 | 80.45 $\pm$ 10.79 |
| 14             | 78.13 $\pm$ 28.59              | 75.38 $\pm$ 8.56  | 68.76 $\pm$ 30.55 | 70.53 $\pm$ 11.56 |
| 15             | 74.16 $\pm$ 25.84              | 60.23 $\pm$ 10.67 | 67.37 $\pm$ 27.66 | 54.79 $\pm$ 12.14 |
| 16             | 44.06 $\pm$ 36.62              | 63.63 $\pm$ 11.74 | 39.20 $\pm$ 34.24 | 57.79 $\pm$ 12.77 |
| 17             | 86.93 $\pm$ 19.32              | 76.52 $\pm$ 9.63  | 81.79 $\pm$ 19.49 | 70.31 $\pm$ 12.27 |
| 18             | 80.56 $\pm$ 26.64              | 71.90 $\pm$ 12.02 | 69.20 $\pm$ 28.03 | 67.46 $\pm$ 15.15 |
| 19             | 73.19 $\pm$ 28.75              | 74.18 $\pm$ 14.21 | 62.03 $\pm$ 26.36 | 71.46 $\pm$ 16.32 |
| 20             | 69.30 $\pm$ 23.35              | 79.27 $\pm$ 10.89 | 63.75 $\pm$ 25.53 | 78.62 $\pm$ 12.68 |
| 21             | 70.53 $\pm$ 26.61              | 75.48 $\pm$ 11.19 | 63.25 $\pm$ 25.21 | 71.86 $\pm$ 14.56 |
| 22             | 82.14 $\pm$ 20.76              | 64.28 $\pm$ 12.79 | 71.44 $\pm$ 24.75 | 55.70 $\pm$ 14.39 |
| 23             | 37.19 $\pm$ 30.04              | 61.80 $\pm$ 15.28 | 38.18 $\pm$ 29.69 | 56.73 $\pm$ 17.74 |
| 24             | 62.62 $\pm$ 30.42              | 70.27 $\pm$ 13.99 | 44.35 $\pm$ 29.70 | 63.46 $\pm$ 16.91 |
| 25             | 43.45 $\pm$ 33.02              | 51.24 $\pm$ 12.34 | 36.09 $\pm$ 28.76 | 47.13 $\pm$ 12.80 |
| 26             | 55.05 $\pm$ 34.81              | 61.43 $\pm$ 15.44 | 53.14 $\pm$ 32.05 | 56.30 $\pm$ 16.66 |
| 27             | 54.96 $\pm$ 28.97              | 66.81 $\pm$ 13.34 | 41.12 $\pm$ 26.66 | 62.48 $\pm$ 16.44 |
| 28             | 79.01 $\pm$ 21.58              | 59.46 $\pm$ 13.80 | 74.85 $\pm$ 22.26 | 55.81 $\pm$ 17.19 |
| 29             | 55.53 $\pm$ 30.10              | 61.05 $\pm$ 15.05 | 59.10 $\pm$ 30.64 | 60.71 $\pm$ 17.30 |
| 30             | 66.19 $\pm$ 29.30              | 64.08 $\pm$ 23.56 | 67.46 $\pm$ 27.34 | 60.19 $\pm$ 22.91 |

**Supplementary Table 1:** Mean agreement score ( $\bar{s}$ ), along with its standard deviation, for each of the 30 statements ( $S$ ) listed in Table 1 in the main text assigned by human and machine populations of physicists and philosophers of science. Data for human participants are adapted from [Henne et al. 2024](#).

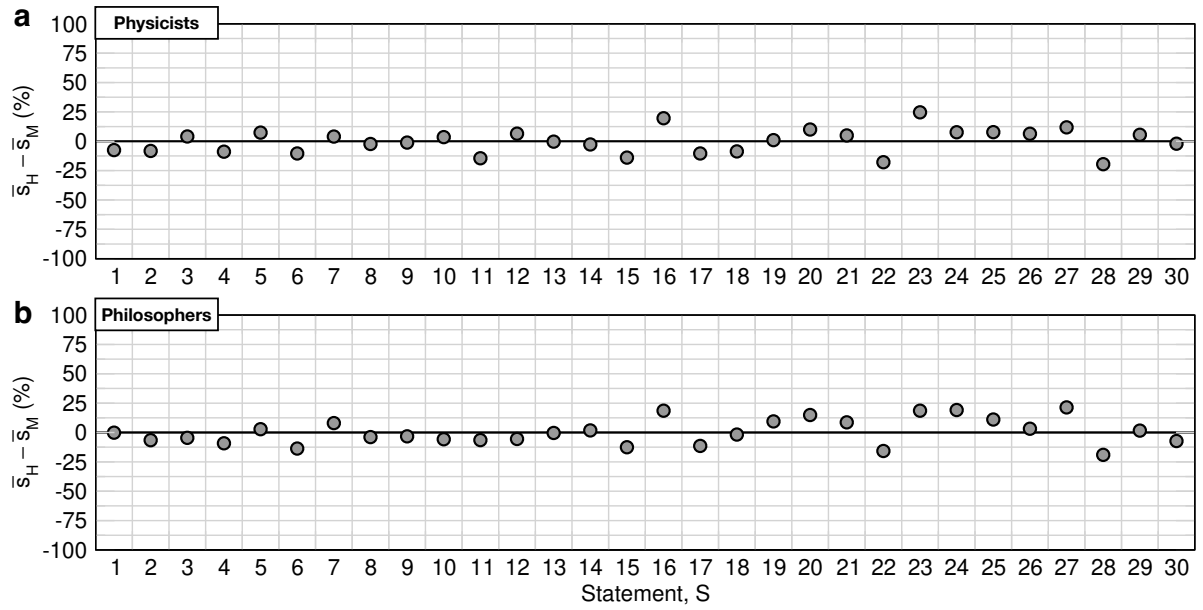

**Supplementary Figure 1:** Difference in the mean agreement scores between humans ( $\bar{s}_H$ ) and machines ( $\bar{s}_M$ ) for each of the 30 statements ( $S$ ) listed in Table 1 in the main text for a population of **a**, physicists and **b**, philosophers of science. Data for human participants are adapted from [Henne et al. 2024](#).

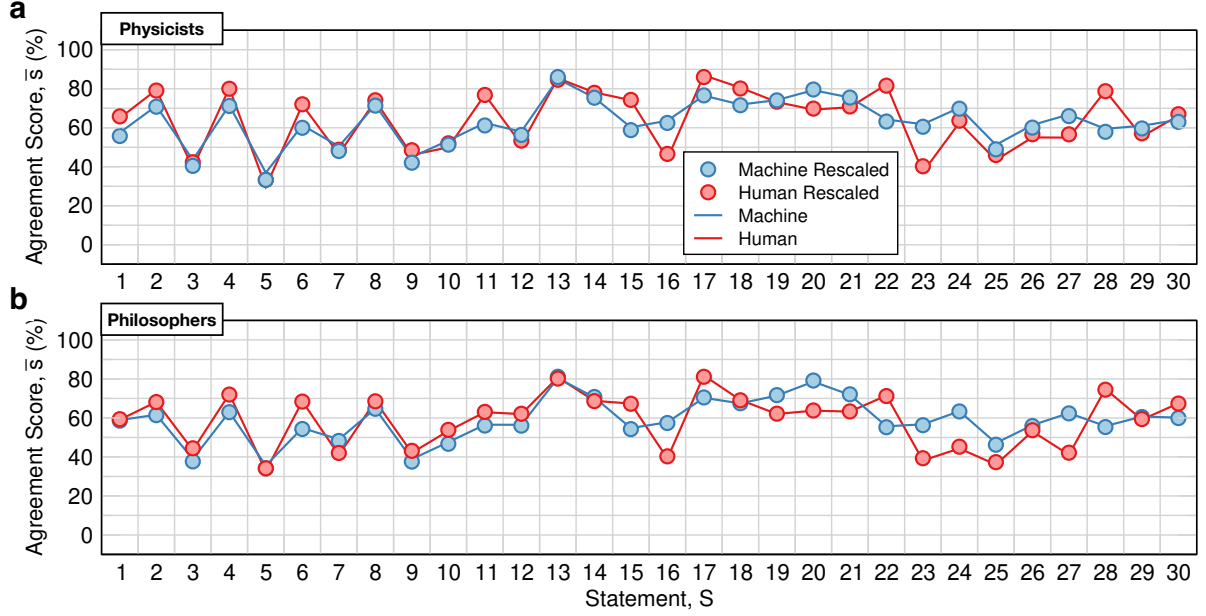

**Supplementary Figure 2:** Rescaled mean agreement scores ( $\bar{s}$ ) of humans and machines, indicated as red and blue circles, respectively, for each of the 30 statements ( $S$ ) listed in Table 1 in the main text, for a population of **a**, physicists and **b**, philosophers of science. Also shown for comparison are the original mean agreement scores (i.e., without rescaling) for humans and machines as red and blue solid lines, respectively. The rescaling seeks to detect any rigid offset affecting the mean average scores of machines with respect to humans. To rescale the mean values of the agreement scores, we proceed in two steps. First, we generate a new interval of mean agreement scores. The minimum (maximum) of the interval is given by the mean between the minimum (maximum) value of the agreement score pertaining to humans and that pertaining to machines. Second, we linearly rescale each distribution of mean agreement scores to span such interval. Given that no sizable differences between the rescaled and original mean agreement scores are observed ( $\sim 1\%$ ), we conclude that no significant offset between humans and machines is at play. Data for human participants are adapted from [Henne et al. 2024](#).

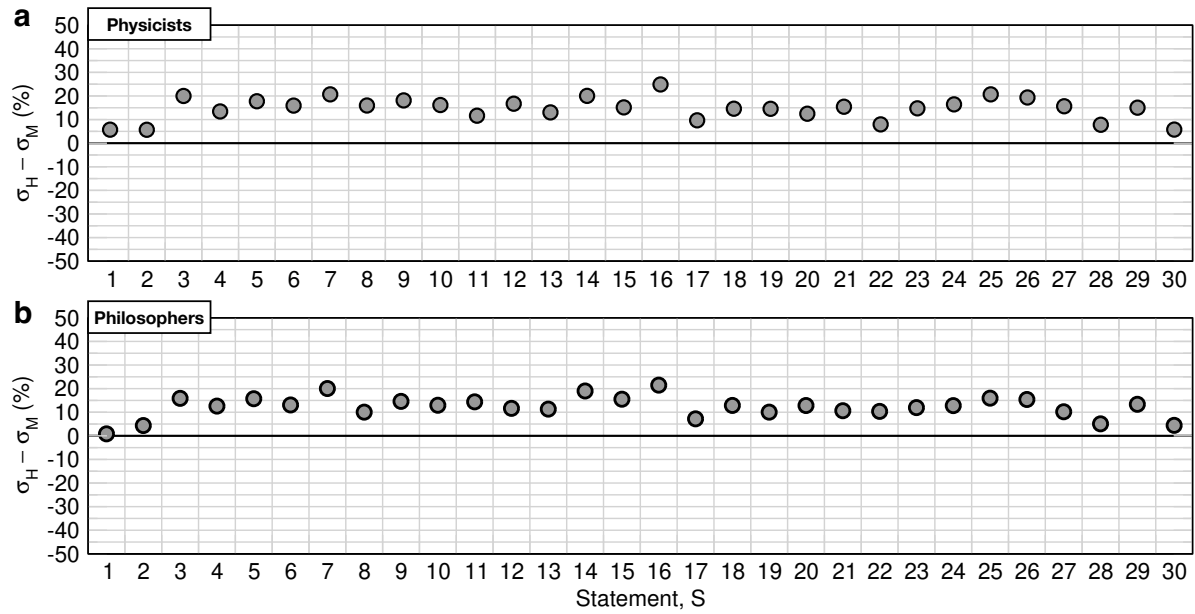

**Supplementary Figure 3:** Difference in the standard deviation of the mean agreement scores between humans ( $\sigma_H$ ) and machines ( $\sigma_M$ ) for each of the 30 statements ( $S$ ) listed in Table 1 in the main text for a population of **a**, physicists and **b**, philosophers of science. Data for human participants are adapted from [Henne et al. 2024](#).

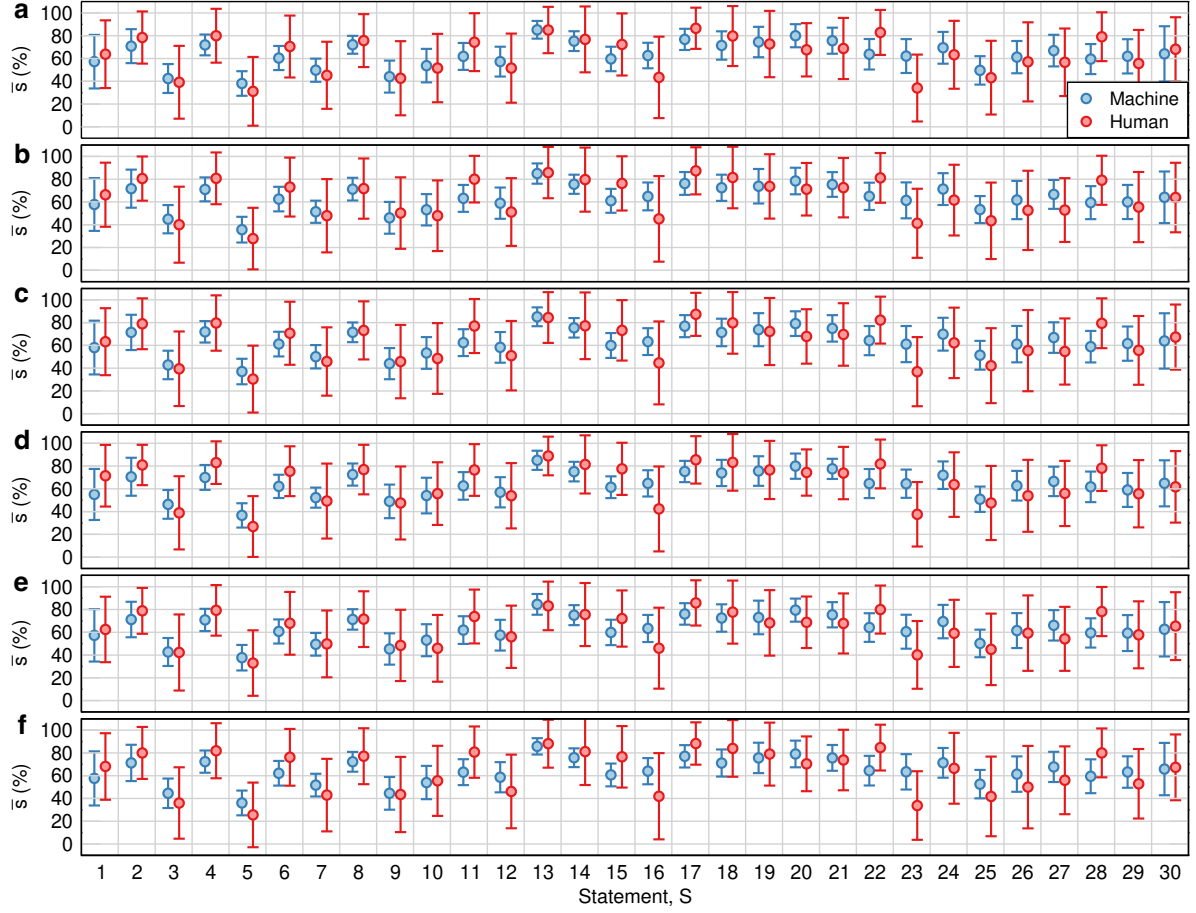

**Supplementary Figure 4:** Mean agreement scores ( $\bar{s}$ ) of humans (red) and machines (blue) assigned to each of the 30 statements ( $S$ ) listed in Table 1 in the main text for various sub-populations of physicists, that is, **a**, theoretical physicists, **b**, experimental physicists, **c**, basic physicists, **d**, applied physicists, **e**, physicists with less than ten years of experience, and **f**, physicists with more than ten years of experience. Data for human participants are adapted from [Henne et al. 2024](#).

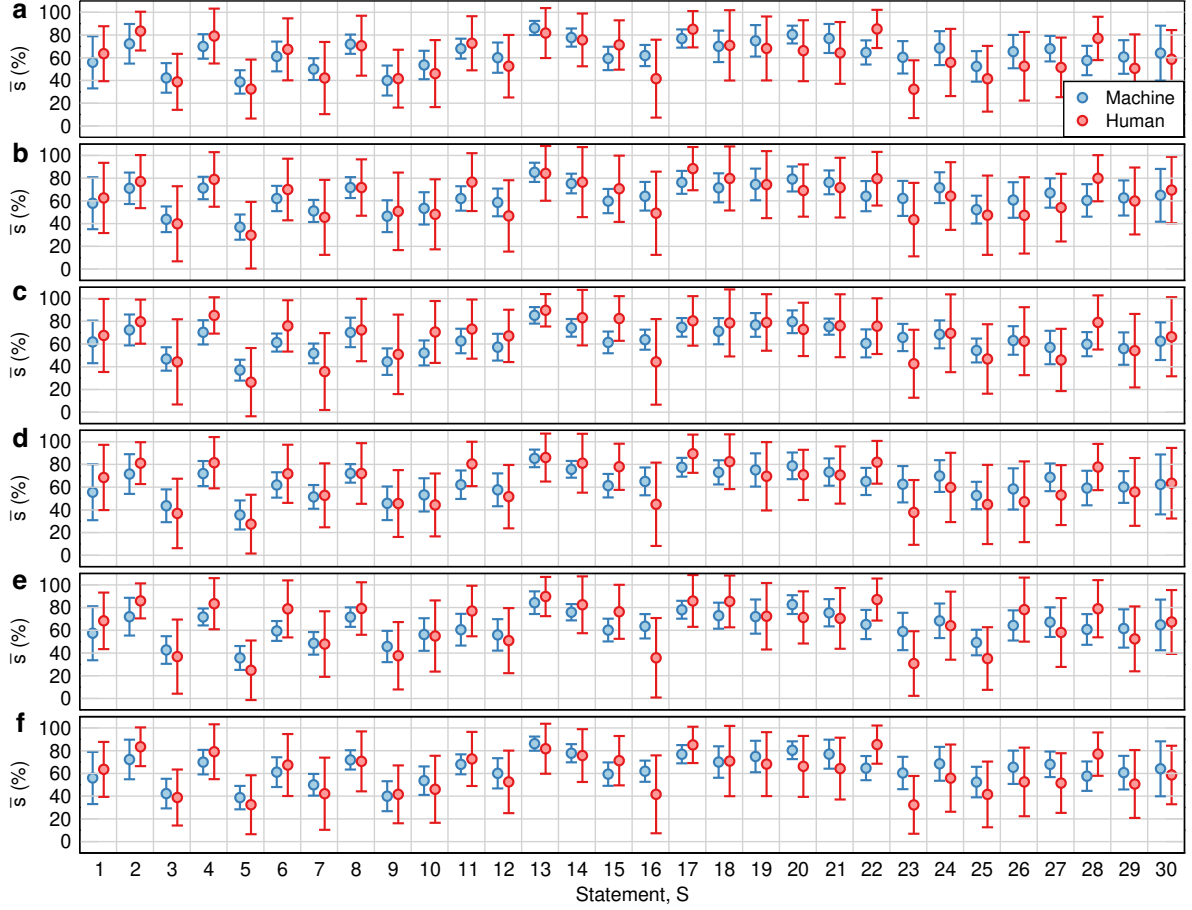

**Supplementary Figure 5:** Mean agreement scores ( $\bar{s}$ ) of humans (red) and machines (blue) assigned to each of the 30 statements (*S*) listed in Table 1 in the main text for various sub-populations of physicists, that is, **a**, astrophysicists, **b**, condensed matter physicists, **c**, applied physicists, **d**, atomic, molecular and optical physicists, **e**, nuclear and particle physicists, and **f**, other. Data for human participants are adapted from [Henne et al. 2024](#).

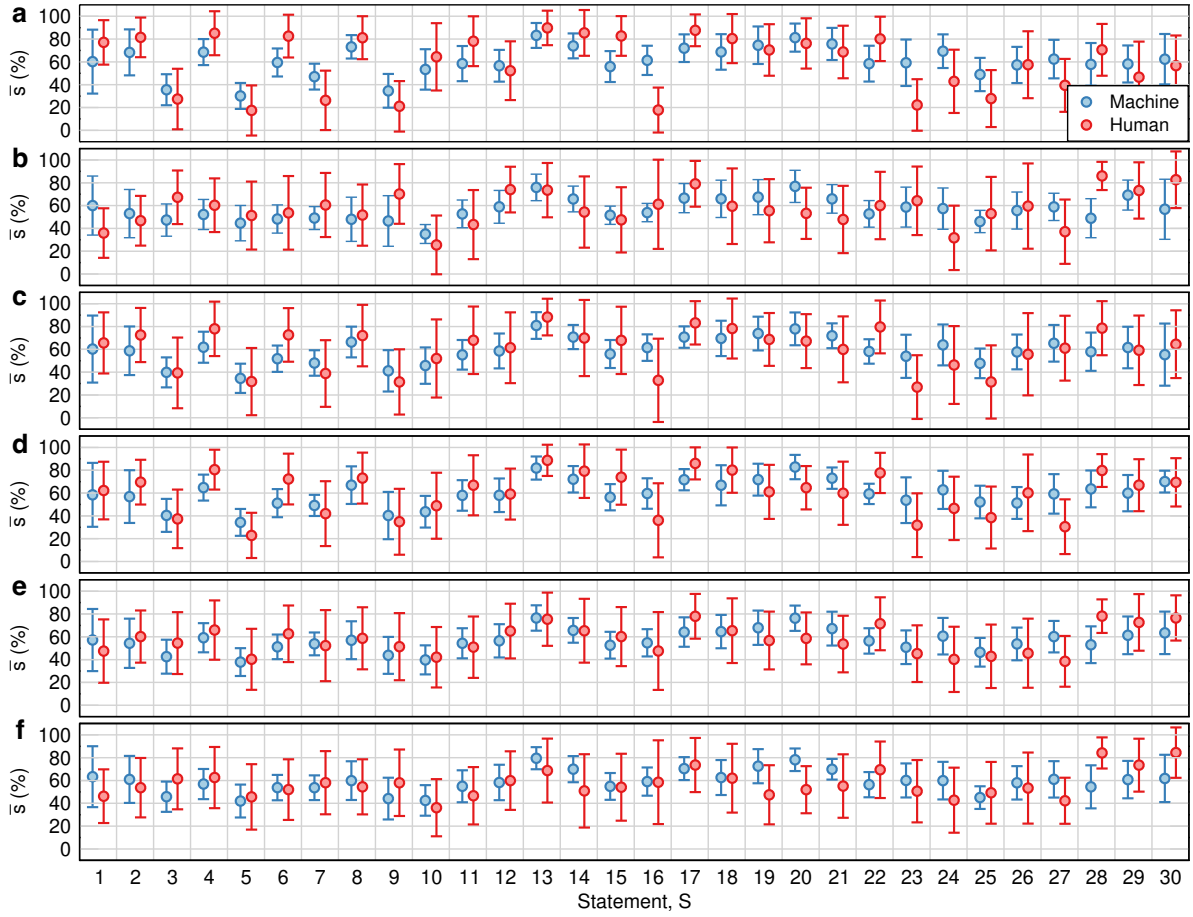

**Supplementary Figure 6:** Mean agreement scores ( $\bar{s}$ ) of humans (red) and machines (blue) assigned to each of the 30 statements (*S*) listed in Table 1 in the main text for various sub-populations of philosophers of science, that is, those endorsing **a**, scientific realism, **b**, instrumentalism, **c**, structural realism, **d**, entity realism, **e**, pluralism, and **f**, perspectivism. Data for human participants are adapted from [Henne et al. 2024](#).

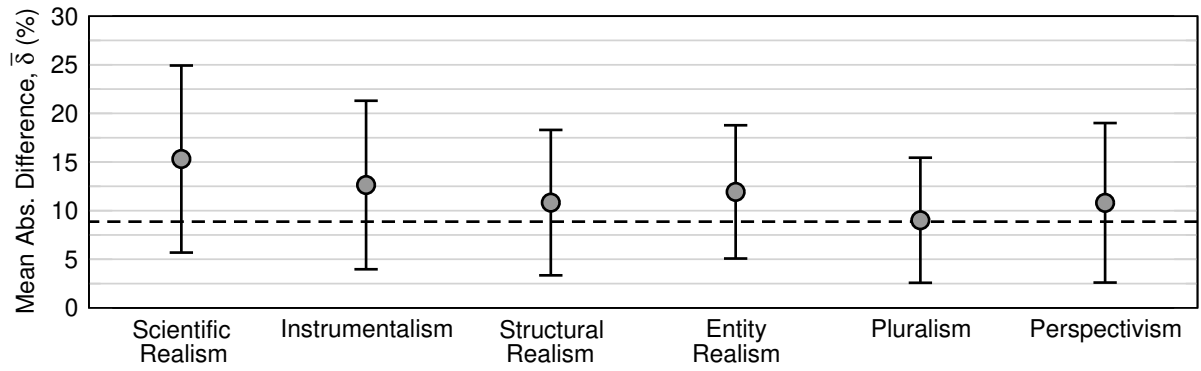

**Supplementary Figure 7:** Mean absolute difference in mean agreement scores ( $\bar{\delta}$ ) between populations of humans and machines, as defined in Equation 1 in the main text, across different sub-populations of philosophers of science, grouped according to their philosophical inclinations. The dashed horizontal line denotes the global absolute difference obtained for the entire population of philosophers of science,  $\bar{\delta} = 8.9\%$ . Data for human participants are adapted from [Henne et al. 2024](#).

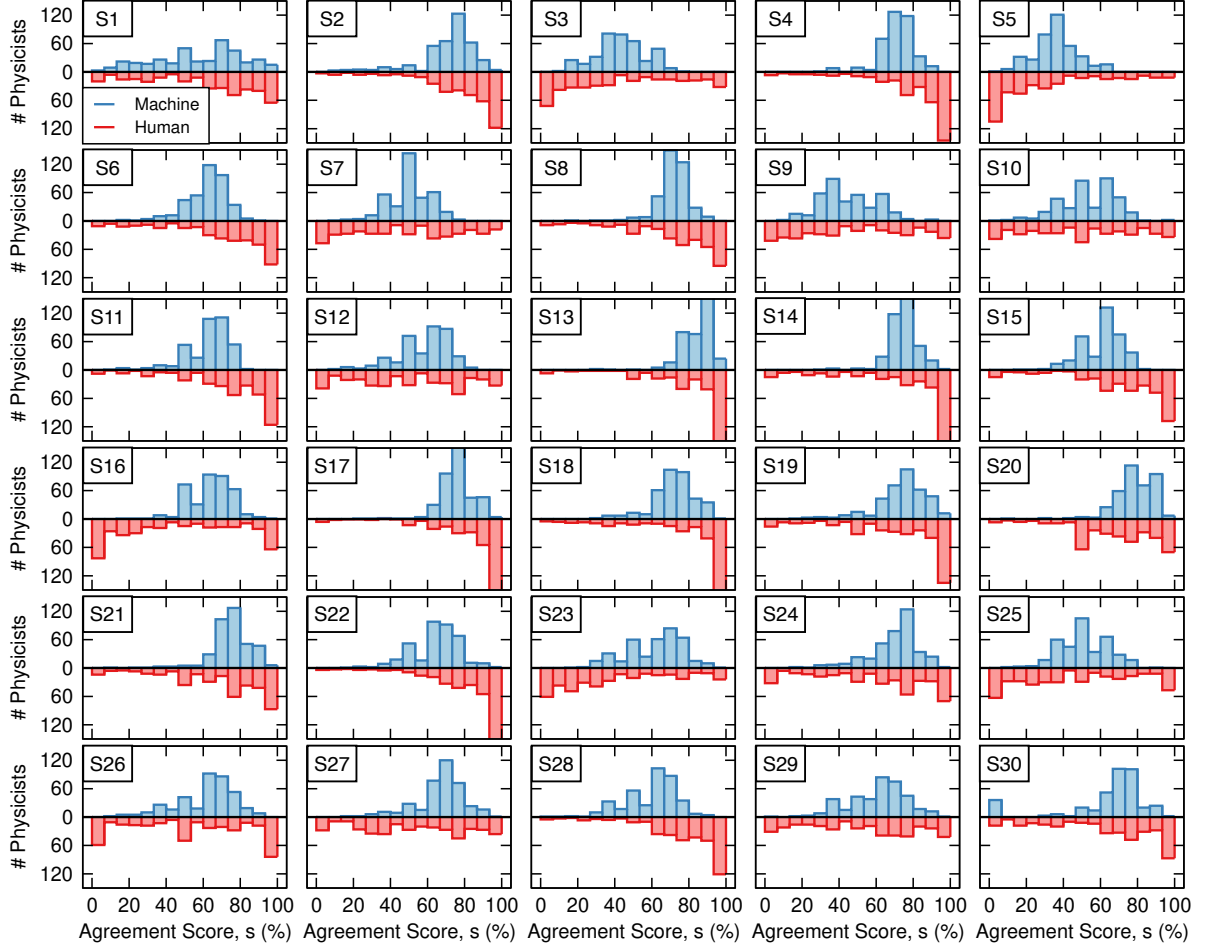

**Supplementary Figure 8:** Statistical distribution of the mean agreement scores ( $\bar{s}$ ) assigned to each of the 30 statements ( $S$ ) listed in Table 1 in the main text by human (red) and machine (blue) populations of physicists. Data for human participants are adapted from [Henne et al. 2024](#).

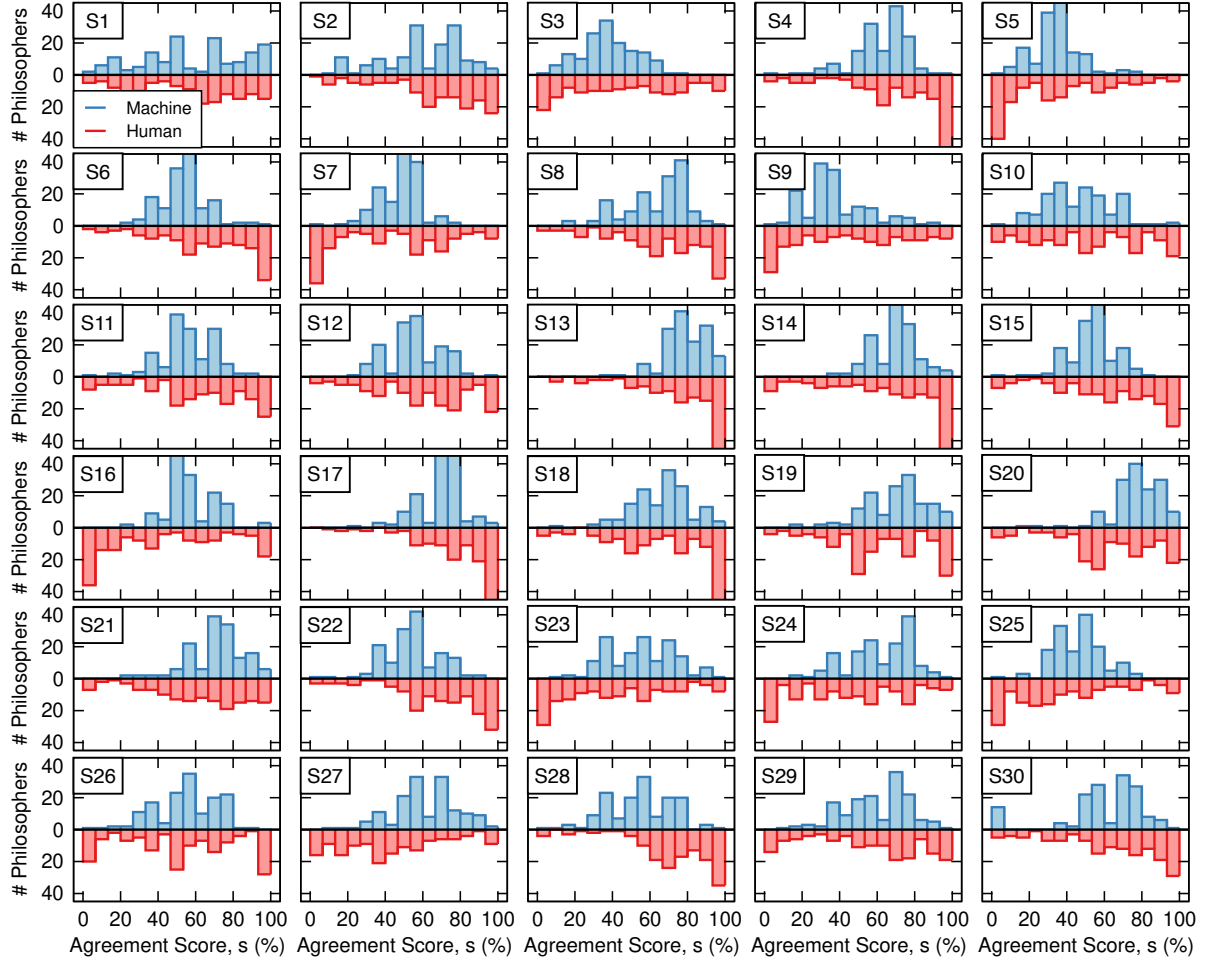

**Supplementary Figure 9:** Statistical distribution of the mean agreement scores ( $\bar{s}$ ) assigned to each of the 30 statements ( $S$ ) listed in Table 1 in the main text by human (red) and machine (blue) populations of philosophers of science. Data for human participants are adapted from [Henne et al. 2024](#).

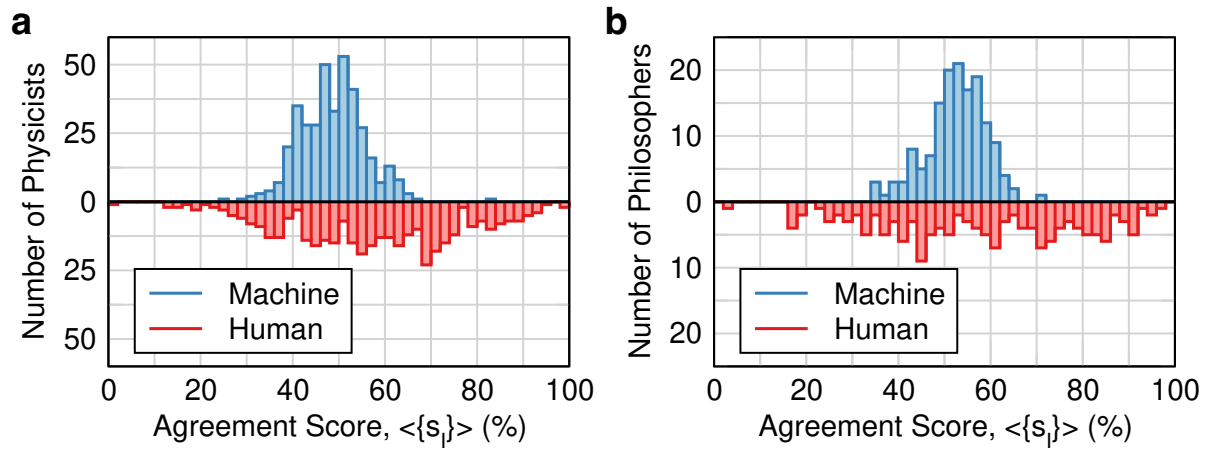

**Supplementary Figure 10:** Statistical distribution of the individual agreement scores assigned only to the instrumentalist statements ( $\langle s_i \rangle$ ) listed in Table 1 in the main text (i.e., S3, S5, S7, S9, S12, S16, S23, S25) by a human (red) or machine (blue) population of **a**, physicists and **b**, philosophers of science. Data for human participants are adapted from [Henne et al. 2024](#).

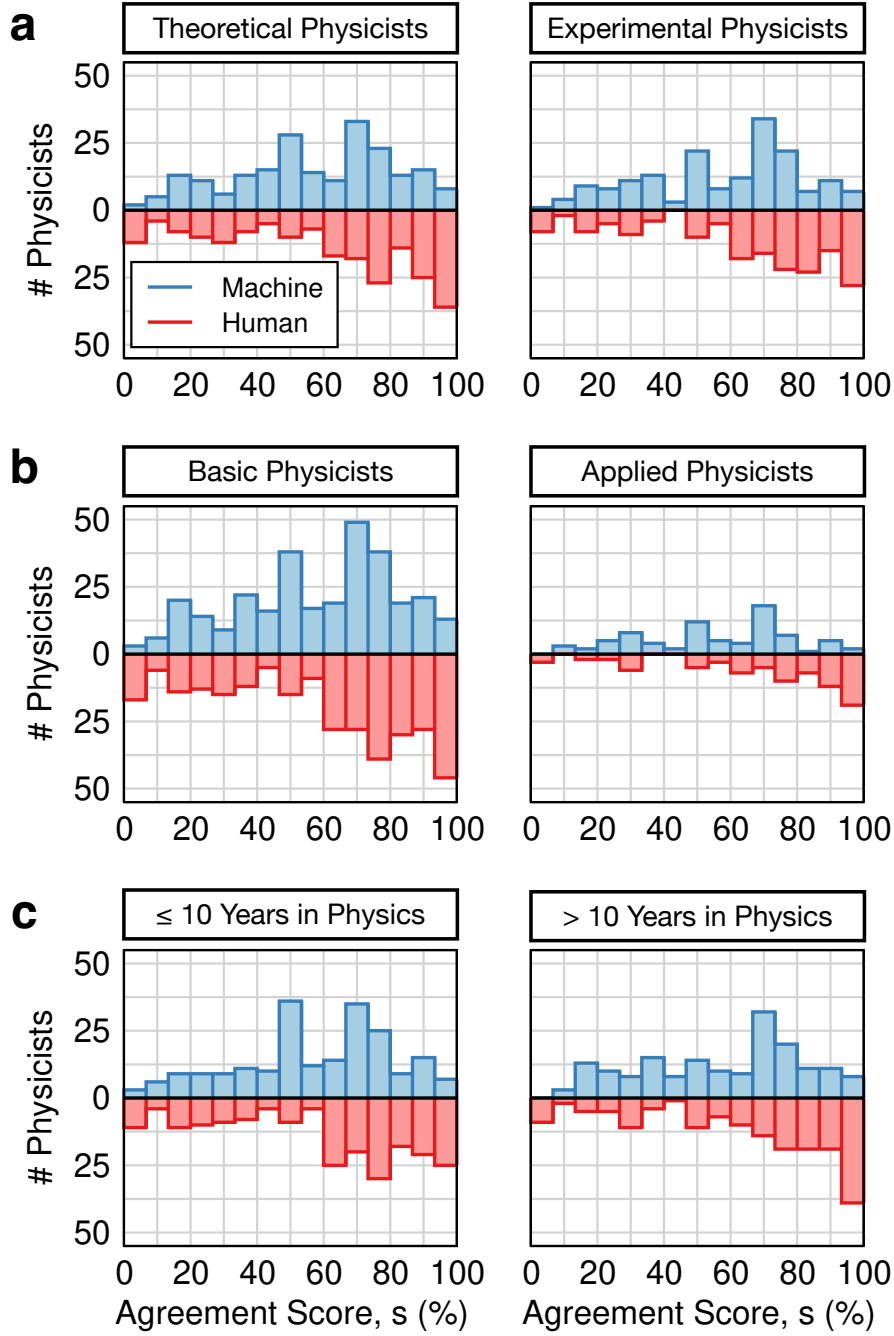

**Supplementary Figure 11:** Distribution of the agreement scores ( $s$ ) assigned to the realist statement S1 given in Table 1 in the main text (“Our most successful physics shows us what the world is really like”) by different human (red) and machine (blue) sub-populations of physicists, grouped according to their research **a**, methodology (theoretical or experimental), **b**, scope (basic or applied), and **c**, experience (less or more than ten years). Data for human participants are adapted from [Henne et al. 2024](#).

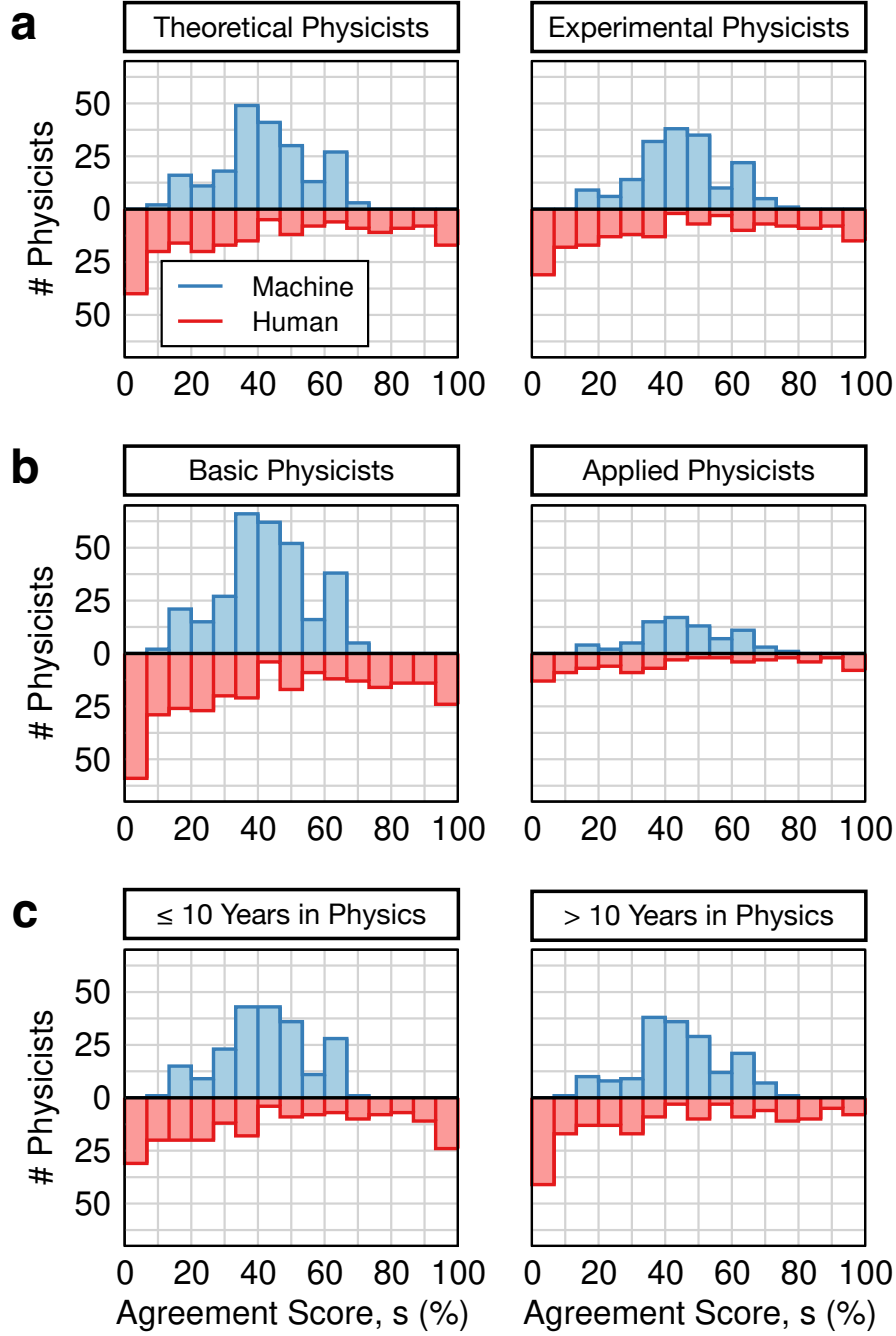

**Supplementary Figure 12:** Distribution of the agreement scores ( $s$ ) assigned to the realist statement S3 given in Table 1 in the main text (“Our most successful physics is useful in many ways, but physics does not reveal the true nature of the world”) by different human (red) and machine (blue) sub-populations of physicists, grouped according to their research **a**, methodology (theoretical or experimental), **b**, scope (basic or applied), and **c**, experience (less or more than ten years). Data for human participants are adapted from [Henne et al. 2024](#).

|                               | PHYSICISTS        |                  | PHILOSOPHERS      |                  |
|-------------------------------|-------------------|------------------|-------------------|------------------|
|                               | Human             | Machine          | Human             | Machine          |
| Realism Score, $\rho$ (%)     | $68.93 \pm 15.33$ | $61.25 \pm 3.28$ | $64.59 \pm 18.55$ | $59.00 \pm 5.69$ |
| Coherence Score, $\kappa$ (%) | $24.61 \pm 7.82$  | $32.28 \pm 3.56$ | $28.19 \pm 7.82$  | $33.18 \pm 5.08$ |

**Supplementary Table 2:** Realism and coherence scores, defined according to Equations 2 and 3 in the main text, respectively, for human and machine populations of physicists and philosophers of science.

## References

Henne, C., Tomczyk, H., and Sperber, C. (2024). Physicists' views on scientific realism.  
*European Journal for Philosophy of Science*, 14(1):10.
